# Supplementary material for: Curve Reconstruction via the Global Statistics of Natural Curves
Source: arXiv:1711.03172 ancillary file (2018-06-13)
Supplement: Supplementary file 1 [file supp.pdf]

# Supplementary Material


## Abstract

*Additional material is provided, including technical details and further reconstruction result. The shown examples cover the space of configurations under the assumptions that curves are invariant to translations, rotations, mirror reflections, and scaling.*


## 1. Scaling of curves

The accurate generation of curves requires to collect enough samples with the same inducer configuration for an accurate estimation of the mean. To increase the number of available samples we also employ fragments with nearly identical configurations (up to scaling if assuming scale invariance) by transforming them so that their end point $\mathbf{q_{xy}}$ exactly matches $\mathbf{p_{xy}}$. To do so, fragments are rotated such that $\mathbf{q_{xy}}$ is placed on the Y axis, scaled across both axes such that $\|\mathbf{q_{xy}}\| = \|\mathbf{p_{xy}}\|$, and then rotated back so that $\mathbf{q_{xy}} = \mathbf{p_{xy}}$. More formally, curve points $x_i$ are transformed such that

$$x_i' = R_{\theta_2} \frac{\|\mathbf{p_{xy}}\|}{\|\mathbf{q_{xy}}\|} R_{\theta_1} x_i \ , \tag{1}$$

where $R_\theta$ is the rotation matrix with some angle $\theta$, $\theta_1$ is negative the angle between $q_{xy}$ and the Y axis, and $\theta_2$ is the angle between $p_{xy}$ and the Y axis. We note that at this stage all fragments end in the bottom half of the coordinate system, so $p_y \leq 0$ and $q_y \leq 0$.

## 2. Initial reconstructions based on the mean curve

Initial reconstructions of different end point configurations based on the mean curve are shown in Figure 1.

## 3. Comparison of reconstructions

Comparison of reconstruction methods can be seen in Figure 2 for configurations with end point orientations in $[0, \frac{3\pi}{4}]$, and in Figure 3 for configurations with end point orientations in $[\pi, \frac{7\pi}{4}]$.

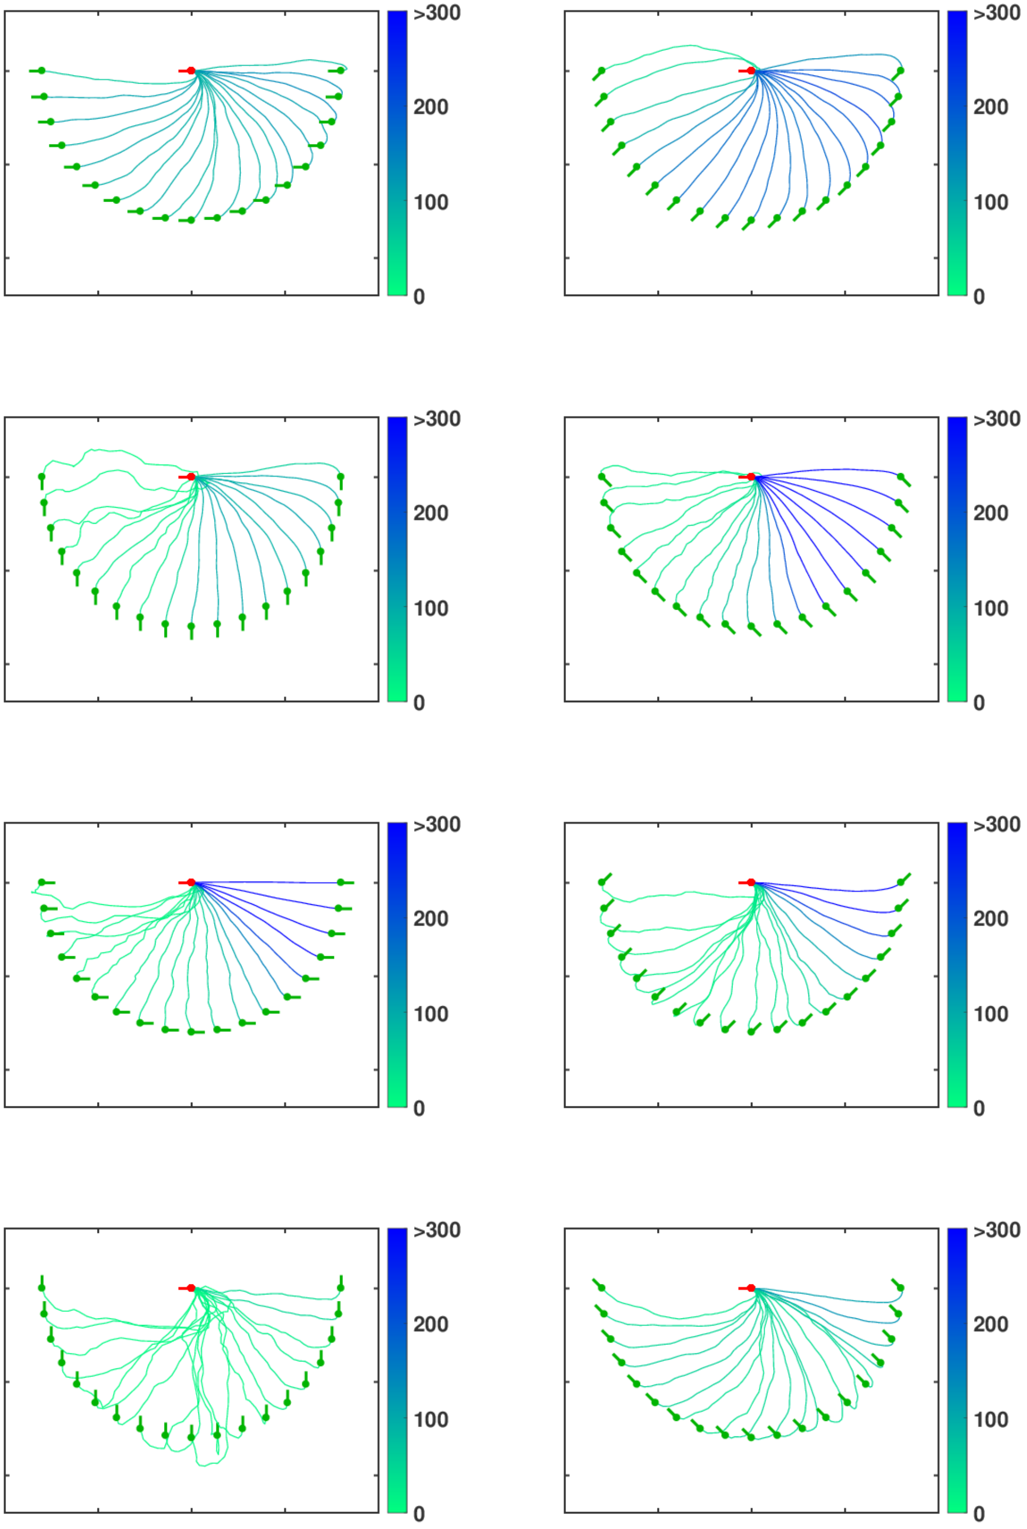


Figure 1. Initial reconstructions based on the mean curve, where curve colors represent the number of fragments used for their generation (darker colors correspond to larger number of ground truth fragments). All inducers in this case are 80 pixels apart. Note how larger sample sets allow more intuitive reconstructions.

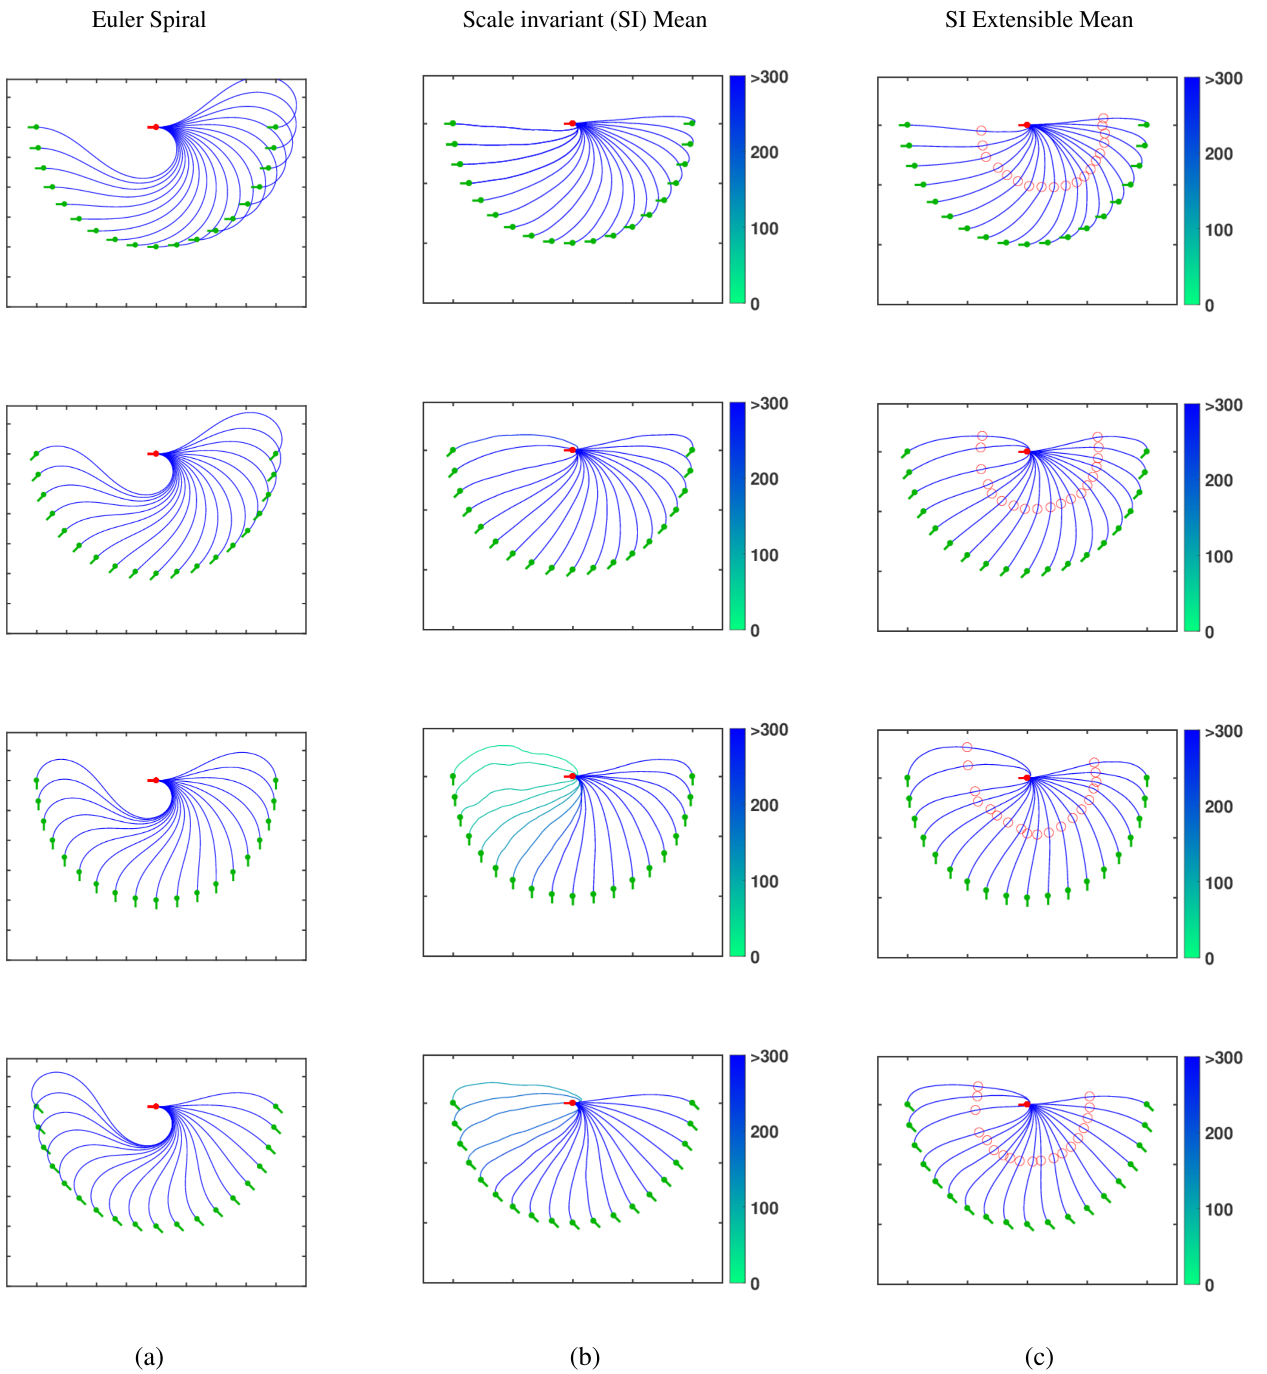


Figure 2. Reconstruction results for curves with end point orientations in $[0, \frac{3\pi}{4}]$ based on (a) Euler spiral, (b) scale invariant mean curve, and (c) extensible and scale invariant mean curve, where darker curve colors represents a larger number of samples from which the curve was calculated. Red circles in (c) mark the points in which two reconstructions are connected to a single curve.

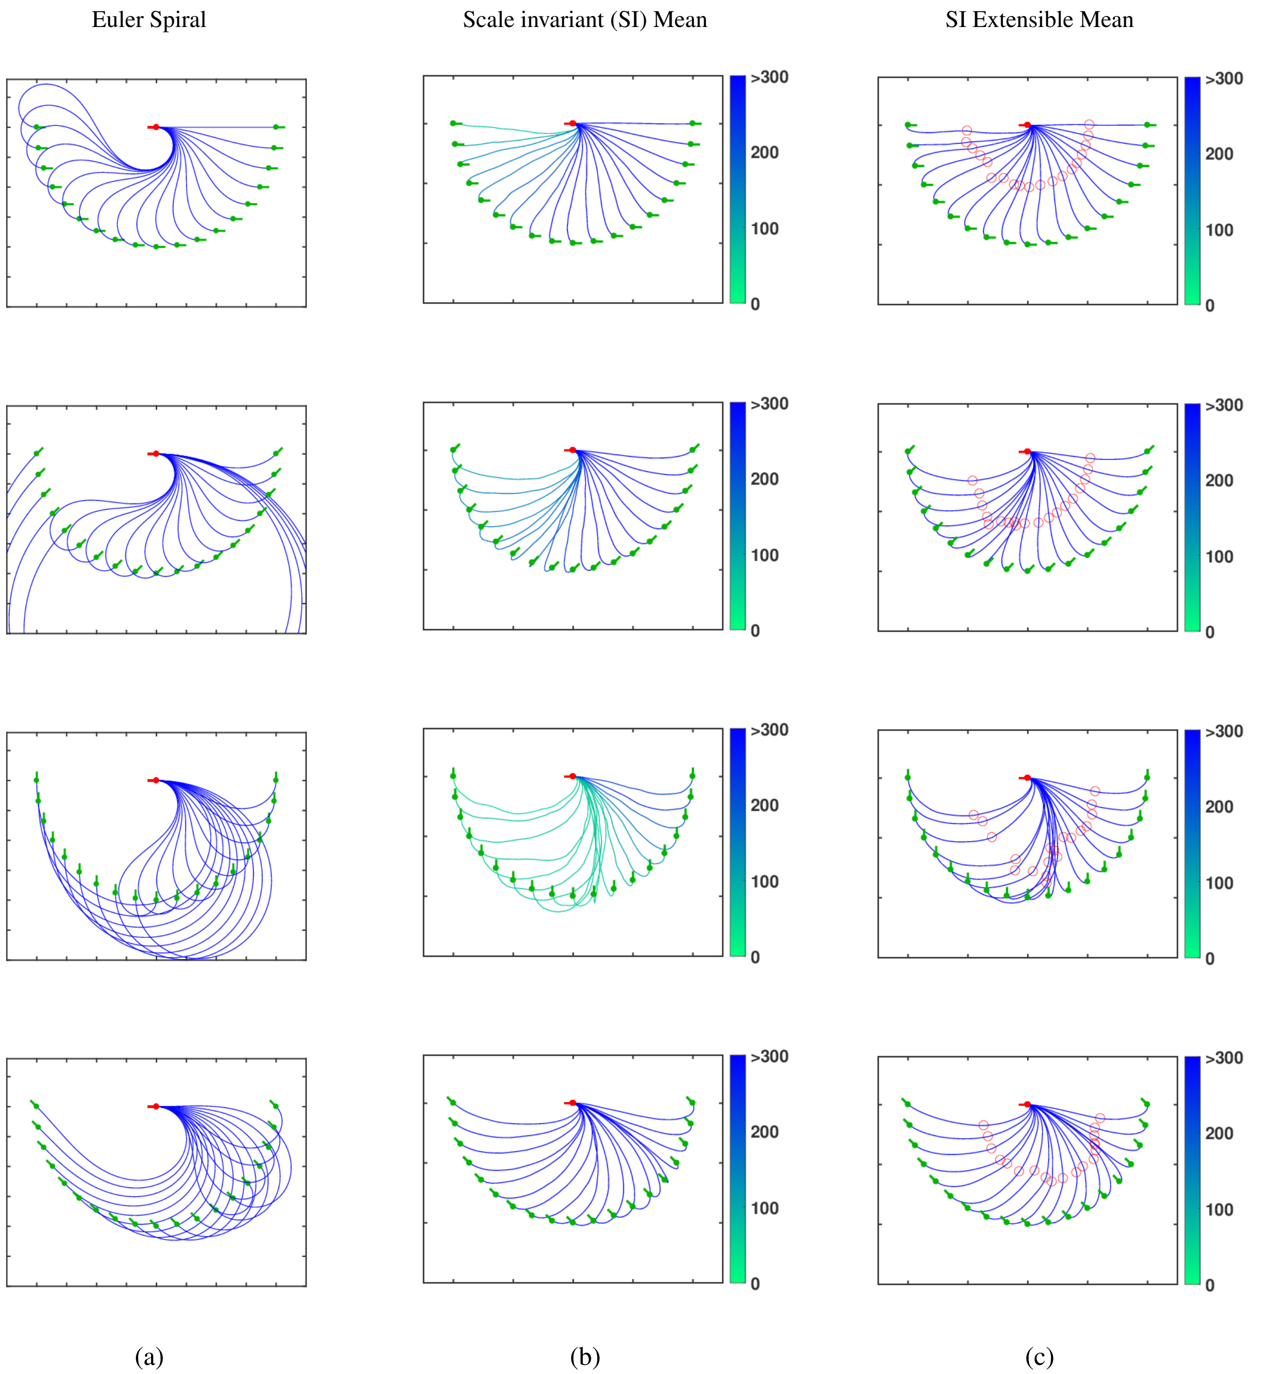


Figure 3. Reconstruction results for curves with end point orientations in $[\pi, \frac{7\pi}{4}]$ based on (a) Euler spiral, (b) scale invariant mean curve, and (c) extensible and scale invariant mean curve, where darker curve colors represents a larger number of samples from which the curve was calculated. Red circles in (c) mark the points in which two reconstructions are connected to a single curve.
